# Supplementary material for: Concave likelihood-based regression with finite-support response variables
Source: arXiv:2203.04582 ancillary file (2022-09-11)
Supplement: Supplementary file 1 [file finite_regr_suppl.pdf]

# Supporting information for “Concave likelihood-based regression with finite-support response variables” by Ekvall and Bottai

Karl Oskar Ekvall<sup>\*,†</sup>   Matteo Bottai<sup>\*</sup>  
`k.ekvall@ufl.edu`   `matteo.bottai@ki.se`

<sup>\*</sup>Division of Biostatistics, Institute of Environmental Medicine, Karolinska Institutet

<sup>†</sup>Department of Statistics, University of Florida

This note contains additional results and technical details for the article “Concave likelihood-based regression with finite-support response variables”. For brevity, that article is referred to as “the main text” in what follows.

## Web Appendix A

### A.1 Depression screening questionnaire data example

We consider the patient health questionnaire (Kroenke and Spitzer, 2002) of the National Health and Nutrition Examination Survey (NHANES). Briefly, patients answer 9 questions on depression symptoms, scoring each question 0, 1, 2, or 3. The outcome of interest here is the cumulative score, taking values in  $\{0, 1, \dots, 27\}$ , which is often used as a screening tool; higher scores correspond to a stronger indication of depression.

It is common to model data like these using linear models, effectively ignoring the discrete and bounded nature of the response. Here we instead consider a model consistent with the observed data. To illustrate, suppose we are interested in whether there is a difference between male and female patients and whether age has an effect on the outcome. Inspecting a histogram of the cumulative scores (Web Figure A), we note an indication the outcome is

right-skewed with substantial mass at low scores. Based on this we consider a model which says the score  $Y_i$  for the  $i$ th patient has mass function

$$f_{\boldsymbol{\theta}}(y_i) = \exp[-\{y_i \exp(-\mathbf{x}_i^{\top} \boldsymbol{\beta} / \sigma)\}^{\sigma}] - \exp[-\{(y_i + 1) \exp(-\mathbf{x}_i^{\top} \boldsymbol{\beta} / \sigma)\}^{\sigma}],$$

with  $y_i + 1$  replaced by  $\infty$  if  $y_i = 27$ . The parameter is  $\boldsymbol{\theta} = [\sigma, \boldsymbol{\beta}^{\top}]^{\top}$  and  $\mathbf{x}_i \in \mathbb{R}^3$  is a vector with a one in the first element (an intercept), age in the second, and an indicator for male in the third. This mass function corresponds to interval-censoring of a latent variable with Weibull distribution, which specializes to the exponential distribution with mean  $\exp(\mathbf{x}^{\top} \boldsymbol{\beta})$  if the scale parameter  $\sigma = 1$ .

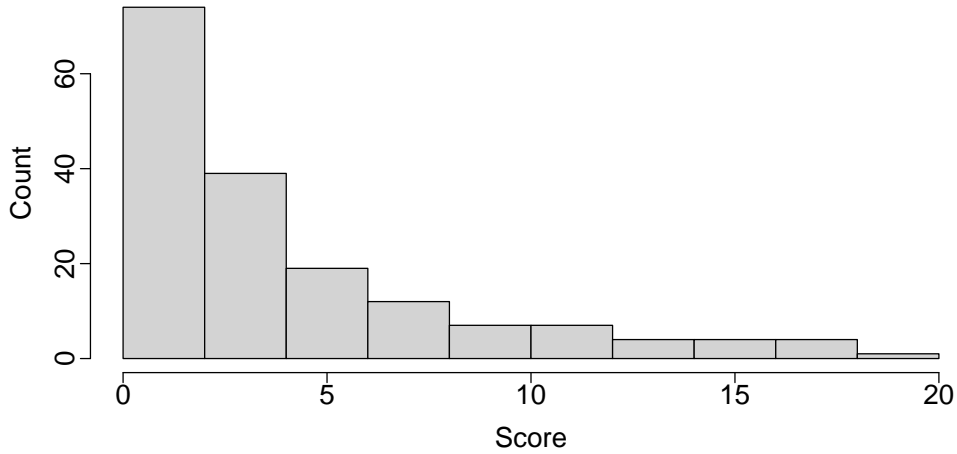

Web Figure A: Histogram of cumulative scores

There are 171 complete observations included in the analysis, 79 males and 92 females. The median age is 19 years. Web Table A shows results from fitting the model. The reported standard errors are square roots of diagonal entries of the inverse of the observed Fisher information matrix. The  $p$ -values are based on a normal approximation and are for the null hypotheses that the scale is one and the regression coefficients are zero. The output indicates male is an important predictor, with males on average scoring lower. We note the scale parameter is significantly different from one, so the exponential distribution is not appropriate in this case.

Web Table A: Interval-censored Weibull regression

|            | Scale       | Intercept | Age   | Male   |
|------------|-------------|-----------|-------|--------|
| Est.       | 0.74        | 0.29      | 0.083 | -0.31  |
| S.E.       | 0.042       | 1.9       | 0.098 | 0.11   |
| $p$ -value | $< 10^{-9}$ | 0.88      | 0.40  | 0.0055 |

Web Figure B shows the estimated mass functions, separately for males and females and with age held fixed at its sample median of 19. The estimated probabilities indicate both males and females are most likely to score roughly in the range 1–5. However, the estimated probabilities for males are higher than those for females for scores 0–4, while for scores 5–27 they are lower than those for females.

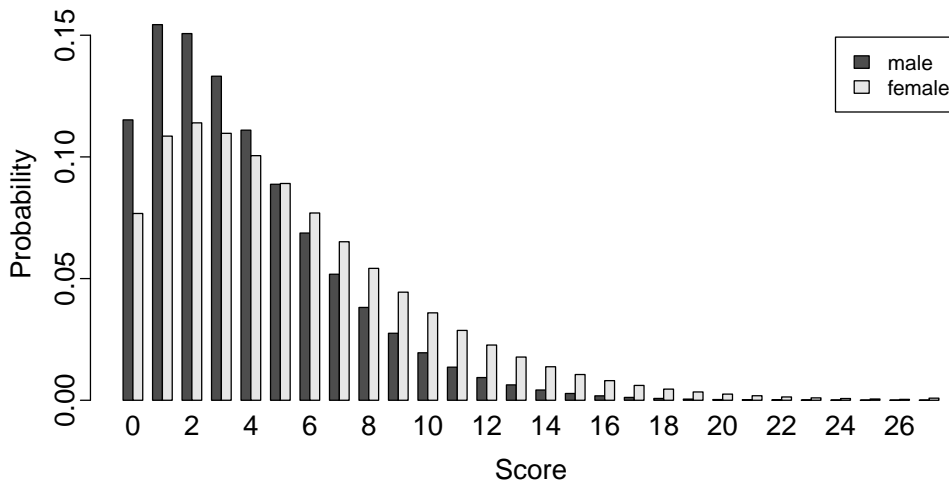

Web Figure B: Estimated probabilities for cumulative scores at age 19

## A.2 Diabetes data example

The R package `glmnetcr` (Archer and Williams, 2012) provides a microarray dataset on  $n = 24$  males, each of which were classified as normal control ( $Y_i = 1$ ), having impaired fasting glucose ( $Y_i = 2$ ), or having Type II diabetes ( $Y_i = 3$ ). The predictors comprise 11,067 gene expression measurements, standardized to have sample mean zero and sample variance one, and interest is in which of these are important for modeling or predicting the response.

With  $R$  the standard normal cumulative distribution function, we consider the model

$$f_{\boldsymbol{\theta}}(y_i) = \begin{cases} R(\alpha_1 + \mathbf{x}_i^\top \boldsymbol{\beta}) & y_i = 1 \\ R(\alpha_2 + \mathbf{x}_i^\top \boldsymbol{\beta}) - R(\alpha_1 + \mathbf{x}_i^\top \boldsymbol{\beta}) & y_i = 2 \\ 1 - R(\alpha_2 + \mathbf{x}_i^\top \boldsymbol{\beta}) & y_i = 3, \end{cases}$$

which is a version of the cumulative probability model in Example 1 in the main text with added predictors. In other words, it is an ordinal probit regression model. The parameter is  $\boldsymbol{\theta} = [\boldsymbol{\alpha}^\top, \boldsymbol{\beta}^\top]^\top \in \Theta = \{\boldsymbol{\theta} \in \mathbb{R}^{11070} : \theta_1 \leq \theta_2\}$ . Consider the estimator

$$\hat{\boldsymbol{\theta}}_n^\lambda \in \arg \min_{\boldsymbol{\theta} \in \Theta} \{-n^{-1} \ell_n(\boldsymbol{\theta}; \mathbf{Y}, \mathbf{X}) + \lambda \|\boldsymbol{\beta}\|_1\}.$$

We select  $\lambda$  using ten-fold cross-validation from the set  $\{2^0, \dots, 2^{-10}\}$  and find that  $\lambda = 2^{-7}$  gives the lowest mis-classification rate, 0.067. At this  $\lambda$  there are 17 non-zero coefficients. By far the largest coefficient is that of the predictor `ILMN_1759232`, which corresponds to Insulin receptor substrate 1; this agrees with previous findings (Archer and Williams, 2012). Web Figure C shows a trace plot for the coefficients.

Fitting the model once for every  $\lambda$  in the given sequence took approximately 4 seconds on a MacBook Pro with a 2.6 GHz 6-core Intel Core i7 processor, and running the 10-fold cross-validation took approximately 40 seconds.

### A.3 Breast cancer data example

Web Figure D shows a trace plot referenced in the main text.

## Web Appendix B

Define  $D : \{\mathbf{t} = (t_1, t_2) \in [-\infty, \infty]^2 : t_1 \leq t_2\} \rightarrow [0, 1]$  by  $D(\mathbf{t}) = \int_{t_1}^{t_2} r(w) dw$ . For interior points of the domain, let  $\mathbf{g}(\mathbf{t}) = \nabla \log\{D(\mathbf{t})\}$  and  $\mathbf{H}(\mathbf{t}) = \nabla^2 \log\{D(\mathbf{t})\}$ . Define also the

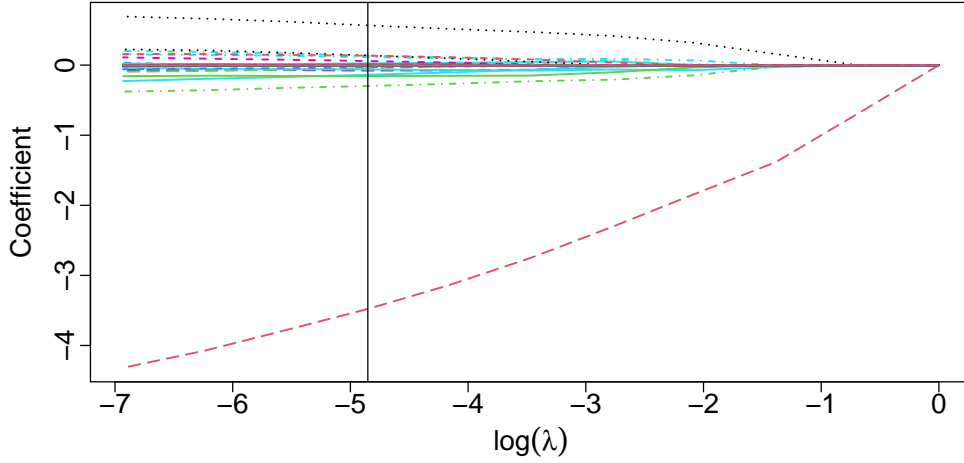

Web Figure C: Trace plot for diabetes data example. The vertical line indicates the selected  $\log(\lambda) = -7 \log(2) \approx -4.85$ .

first element of  $\mathbf{g}(\mathbf{t})$ , and the first row and column of  $\mathbf{H}(\mathbf{t})$ , to vanish when  $t_1$  is infinite. Similarly, the second element of  $\mathbf{g}(\mathbf{t})$  and second row and column of  $\mathbf{H}(\mathbf{t})$  vanish when  $t_2$  is infinite. Finally, when  $t_1 = t_2$ ,  $\mathbf{g}(\mathbf{t}) = \mathbf{0}$  and  $\mathbf{H}(\mathbf{t}) = \mathbf{0}$ . Thus,  $\mathbf{g}$  and  $\mathbf{H}$  are defined on the same domain as  $D$ .

When the log-likelihood is differentiable, its gradient is

$$\nabla \ell_n(\boldsymbol{\theta}; \mathbf{Y}, \mathbf{X}) = \sum_{i=1}^n \mathbf{Z}_i^\top \mathbf{g}(a_i(y_i, \mathbf{x}_i, \boldsymbol{\theta}), b_i(y_i, \mathbf{x}_i, \boldsymbol{\theta})).$$

When the log-likelihood is twice differentiable, its Hessian is

$$\sum_{i=1}^n \mathbf{Z}_i^\top \mathbf{H}(a_i(y_i, \mathbf{x}_i, \boldsymbol{\theta}), b_i(y_i, \mathbf{x}_i, \boldsymbol{\theta})) \mathbf{Z}_i.$$

We overload notation and often simplify  $\mathbf{H}(a_i(y_i, \mathbf{x}_i, \boldsymbol{\theta}), b_i(y_i, \mathbf{x}_i, \boldsymbol{\theta}))$  to  $\mathbf{H}(y_i, \mathbf{x}_i, \boldsymbol{\theta})$  or, when the arguments are clear from context,  $\mathbf{H}_i$ .

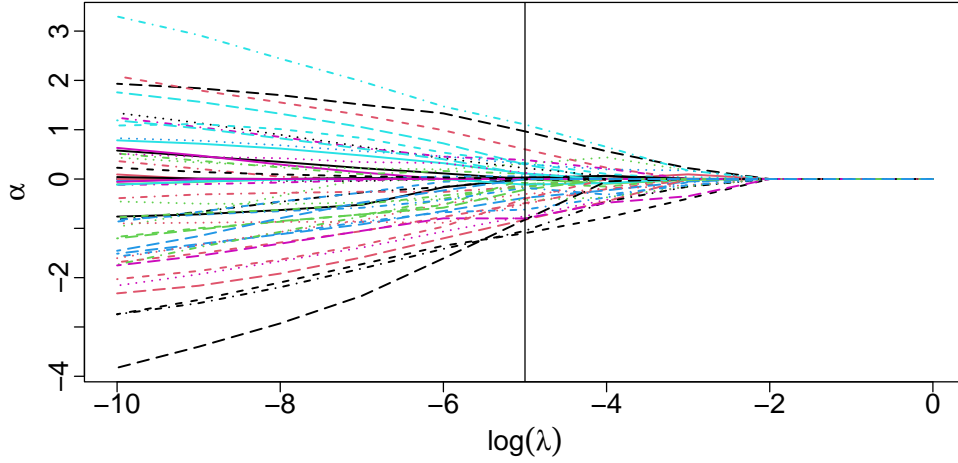

Web Figure D: Trace plot for gene expression coefficients. The vertical line indicates the selected  $\log(\lambda) = -5$ .

## B.1 Concavity of the log-likelihood

**Lemma B.1.** *For any log-concave Lebesgue density  $r$  on  $\mathbb{R}$  the function  $D$  is log-concave. Moreover, if  $r$  is strictly positive and strictly log-concave on an interval  $(a, b)$ ,  $-\infty \leq a < b \leq \infty$ , then  $D$  is strictly log-concave on  $\{\mathbf{t} \in \mathbb{R}^2 : a < t_1 < t_2 < b\}$ .*

*Remark.* The first assertion of the lemma implies the cumulative distribution function  $R$  and the survival function  $1 - R$  are both log-concave. The second assertion implies  $t_1 \mapsto D(t_1, t_2)$  is strictly log-concave on  $(a, t_2)$  and  $t_2 \mapsto D(t_1, t_2)$  is strictly log-concave on  $(t_1, b)$ .

*Proof.* The first assertion follows from (i) the maps  $(t_1, t_2, w) \mapsto \mathbb{I}(t_1 \leq w \leq t_2)$  and  $(t_1, t_2, w) \mapsto r(w)$  are log-concave, (ii) the product of log-concave functions is log-concave, and (iii) integrating out one variable from a log-concave function on  $\mathbb{R}^3$  gives a log-concave function on  $\mathbb{R}^2$  (Prékopa, 1973, Theorem 6).

To prove the strict log-concavity we will use Theorem 4 of Prékopa (1973) in a way similar to the proof of their Theorem 5. Denote  $\mathcal{T} = \{\mathbf{t} \in \mathbb{R}^2 : a < t_1 < t_2 < b\}$ , where  $a < b$  and  $r$  is strictly positive and strictly log-concave on  $(a, b)$ . Note  $\mathcal{T}$  non-empty, convex, and open. Pick  $u, v \in \mathcal{T}$ ,  $u \neq v$ . If  $u_1 \neq v_1$ , define the intervals  $U = [u_1, u_2)$  and  $V = [v_1, v_2)$ . Define

also  $U_1 = [u_1, u_1 + \epsilon]$  and  $V_1 = [v_1, v_1 + \delta]$ , where  $\epsilon > 0$  and  $\delta > 0$  are small enough that  $U_2 = U \setminus U_1$  and  $V_2 = V \setminus V_1$  are non-empty.

We will omit the arguments for the case  $u_1 = v_1, u_2 \neq v_2$  since they are very similar but with the definitions  $U = (u_1, u_2]$ ,  $V = (v_1, v_2]$ ,  $U_1 = [u_2 - \epsilon, u_2]$ , and  $V_1 = [v_2 - \delta, v_2]$ .

Now, with  $R$  denoting the distribution with cumulative distribution function  $R$ , we have  $D(u) = R(U)$ ,  $D(v) = R(V)$ , and

$$D(su + (1 - s)v) = R(sU + (1 - s)V),$$

where for sets addition is in the Minkowski sense and scalar multiplication is elementwise. Thus, we need to show  $R(sU + (1 - s)V) > R(U)^s R(V)^{1-s}$ . By construction,  $U_1$  and  $U_2$  are convex and partition  $U$ ,  $U_1$  is closed and bounded, and both  $U_1$  and  $U_2$  have positive  $R$ -measure. Similar statements apply to  $V_1$ ,  $V_2$ , and  $V$ . This verifies condition a) and Equation (3.5) of Theorem 4 by Prékopa (1973). Condition d) holds because the convex hull of  $U_1 \cup V_1$  is a closed interval contained in  $(a, b)$ . It remains to verify their condition (b) and Equation (3.6).

Observe

$$\begin{aligned} sU_1 + (1 - s)V_1 &= [su_1, s(u_1 + \epsilon)] + [(1 - s)v_1, (1 - s)(v_1 + \delta)] \\ &= [su_1 + (1 - s)v_1, su_1 + (1 - s)v_1 + s\epsilon + (1 - s)\delta] \end{aligned}$$

and

$$\begin{aligned} sU_2 + (1 - s)V_2 &= (s(u_1 + \epsilon), su_2) + ((1 - s)(v_1 + \delta), (1 - s)v_2) \\ &= (su_1 + (1 - s)v_1 + s\epsilon + (1 - s)\delta, su_2 + (1 - s)v_2). \end{aligned}$$

Thus, Equations (3.1) and (3.2) in Prékopa (1973) hold by inspection. To ensure their Equations (3.3) and 3.4 also hold, note that as  $\epsilon, \delta \rightarrow 0$ ,  $sU_1 + (1 - s)V_1$  shrinks towards the

point  $su_1 + (1 - s)v_1$  and  $U_1$  shrinks towards the point  $u_1$ . Thus, they are disjoint for small enough  $\epsilon$  and  $\delta$  because  $u_1 \neq v_1$  and  $s \in (0, 1)$ . Similarly,  $V_1$  and  $sU_1 + (1 - s)V_1$  are disjoint for small enough  $\epsilon$  and  $\delta$  and that verifies Equations (3.3) and (3.4). As argued in the proof of Theorem 5 in Prékopa (1973), their Equation (3.6), which says  $R(U_2)/R(U_1) = R(V_2)/R(V_1)$ , can be made to hold because the left-hand side does not depend on  $\delta$  and tends to infinity as  $\epsilon \rightarrow 0$ , and the right-hand side does not depend on  $\epsilon$  and tends to infinity as  $\delta \rightarrow 0$ . We conclude all the sufficient conditions hold, and hence  $R(sU + (1 - s)V) > R(U)^s R(V)^{1-s}$  as desired.  $\square$

*Proof of Theorem 1.* The non-strict concavity follows from the non-strict log-concavity given by Lemma B.1 and the fact that the composition of a concave and an affine function is concave. To prove the strict part, note continuous differentiability of  $r$  implies  $\nabla^2 \ell_n(\boldsymbol{\theta}; \mathbf{Y}, \mathbf{X})$  exists on every interior point of  $\Theta$ . Thus, it suffices to prove  $\nabla^2 \ell_n(\boldsymbol{\theta}; \mathbf{Y}, \mathbf{X})$  is negative definite (Boyd and Vandenberghe, 2004, p.71). Recall the Hessian is

$$\nabla^2 \ell_n(\boldsymbol{\theta}; \mathbf{Y}, \mathbf{X}) = \sum_{i=1}^n \mathbf{Z}_i^\top \mathbf{H}_i \mathbf{Z}_i.$$

Now, when  $m_i^a$  and  $m_i^b$  are both finite,  $\mathbf{H}_i$  is negative definite by Lemma B.1. For  $y_i$  such that  $m_i^a = -\infty$ , we have that  $\mathbf{z}_i^a = \mathbf{0}$  and hence

$$\mathbf{Z}_i^\top \mathbf{H}_i \mathbf{Z}_i = \mathbf{H}_{22}(y_i, \mathbf{x}_i, \boldsymbol{\theta}) \mathbf{Z}_i^\top \mathbf{Z}_i.$$

Similarly, for  $y_i$  such that  $m_i^b = \infty$  we have

$$\mathbf{Z}_i^\top \mathbf{H}_i \mathbf{Z}_i = \mathbf{H}_{11}(y_i, \mathbf{x}_i, \boldsymbol{\theta}) \mathbf{Z}_i^\top \mathbf{Z}_i.$$

By Lemma B.1,  $\mathbf{H}_{11}$  and  $\mathbf{H}_{22}$  are strictly negative. Thus, we can find an  $\epsilon = \epsilon(\mathbf{Y}, \mathbf{X}, \boldsymbol{\theta}) > 0$

such that

$$\lambda_{\max} \left( \sum_{i=1}^n \mathbf{z}_i^\top \mathbf{H}_i \mathbf{z}_i \right) < \epsilon \lambda_{\max} \left( \sum_{i=1}^n \mathbf{z}_i^\top \mathbf{z}_i \right) < 0,$$

which completes the proof.  $\square$

## B.2 Asymptotics with fixed number of parameters

**Lemma B.2.** *If  $r$  is continuously differentiable, Assumption 1 holds, and  $\|\boldsymbol{\theta}_*\|_1 \leq c_1$ , then for all small enough  $\rho > 0$  there exists an  $\epsilon > 0$  such that for all  $i \in \mathbb{N}$ ,  $\mathbf{x} \in \mathcal{X}$ , and  $\boldsymbol{\theta}$  with  $\|\boldsymbol{\theta} - \boldsymbol{\theta}_*\|_1 \leq \rho$ :*

1.  $\mathbf{H}_{11}(y_i, \mathbf{x}, \boldsymbol{\theta}) \leq -\epsilon$  if  $a_i(y_i, \mathbf{x}, \boldsymbol{\theta}) > -\infty$  and  $b_i(y_i, \mathbf{x}, \boldsymbol{\theta}) = \infty$ ;
2.  $\mathbf{H}_{22}(y_i, \mathbf{x}, \boldsymbol{\theta}) \leq -\epsilon$  if  $a_i(y_i, \mathbf{x}, \boldsymbol{\theta}) = -\infty$  and  $b_i(y_i, \mathbf{x}, \boldsymbol{\theta}) < \infty$ ; and
3.  $\lambda_{\max} \{\mathbf{H}(y_i, \mathbf{x}, \boldsymbol{\theta})\} \leq -\epsilon$  if  $a_i(y_i, \mathbf{x}, \boldsymbol{\theta}) > -\infty$  and  $b_i(y_i, \mathbf{x}, \boldsymbol{\theta}) < \infty$

*Proof.* Continuous differentiability of  $r$  implies  $\mathbf{H}(t_1, t_2)$  is continuous on  $\{\mathbf{t} : t_1 < t_2\}$ ,  $t_1 \mapsto \mathbf{H}_{11}(t_1, \infty)$  is continuous on  $\mathbb{R}$ , and  $t_2 \mapsto \mathbf{H}_{22}(-\infty, t_2)$  is continuous on  $\mathbb{R}$ . Lemma B.1 says the functions are also strictly negative on the given domains. Consider first  $y_i$  such that  $b_i(y_i, \mathbf{x}, \boldsymbol{\theta}) = \infty$ .

$$\begin{aligned} |\boldsymbol{\theta}^\top \mathbf{z}_i^a + m_i^a| &\leq |(\boldsymbol{\theta} - \boldsymbol{\theta}_*)^\top \mathbf{z}_i^a + m_i^a| + |\boldsymbol{\theta}_*^\top \mathbf{z}_i^a| \\ &\leq (1 + \rho)c_2 + c_1c_2 =: c_3, \end{aligned}$$

where the constant  $c_2$  is given by Assumption 1. Now point 1 in the conclusion follows from that  $t_1 \mapsto \mathbf{H}_{11}(t_1, \infty)$  is continuous and strictly negative on the compact  $[-c_3, c_3]$ , and hence attains a strictly negative maximum there. We omit the arguments for the other cases since they are very similar, using for the case where neither endpoint is infinite that  $\mathbf{Z}_i \boldsymbol{\theta} + \mathbf{m}_i$  is, by Assumption 1, contained in a compact set on which  $\lambda_{\max} \{\mathbf{H}(t_1, t_2)\}$  is strictly negative.  $\square$

**Lemma B.3** (Bartlett identities). *If, in Model (1) in the main text, the density  $r$  is strictly positive and continuous and  $\|\mathbf{Z}(y, \mathbf{x})\| < \infty$  for all  $(y, \mathbf{x})$ , then  $\mathbb{E}_{\boldsymbol{\theta}}\{\nabla \ell(\boldsymbol{\theta}; Y, \mathbf{x})\} = 0$  and  $-\mathbb{E}_{\boldsymbol{\theta}}\{\nabla^2 \ell(\boldsymbol{\theta}; Y, \mathbf{x})\} = \text{cov}_{\boldsymbol{\theta}}\{\nabla \ell(\boldsymbol{\theta}; Y, \mathbf{x})\}$  for every  $\mathbf{x}$  and  $\boldsymbol{\theta}$ .*

*Proof.* By a classical argument, it suffices to show we can differentiate twice under the integral in the identity  $\int f_{\boldsymbol{\theta}}(y \mid \mathbf{x}) dy$ , where  $dy$  indicates integration with respect to the measure against which  $Y$  has density  $f_{\boldsymbol{\theta}}(y \mid \mathbf{x})$ . We show it can be done once by showing that for every  $\|\nabla f_{\boldsymbol{\theta}}(y \mid \mathbf{x})\|_1$  is bounded by an integrable function of  $y$  not depending on  $\boldsymbol{\theta}$  (Folland, 2007, Theorem 2.27). In fact, we have

$$\begin{aligned} \|\nabla f_{\boldsymbol{\theta}}(y \mid \mathbf{x})\|_1 &= \|r(b(y, \mathbf{x}, \boldsymbol{\theta}))\mathbf{z}^b - r(a(\boldsymbol{\theta}, y, \mathbf{x}))\mathbf{z}^a\|_1 \\ &\leq |r(b(y, \mathbf{x}, \boldsymbol{\theta}))|\|\mathbf{z}^b\|_1 + |r(a(\boldsymbol{\theta}, y, \mathbf{x}))|\|\mathbf{z}^a\|_1 \\ &\leq c_1, \end{aligned}$$

where  $c_1 < \infty$  depends on neither of  $y$ ,  $\mathbf{x}$ , or  $\boldsymbol{\theta}$ ; and  $\mathbf{z}^a$  and  $\mathbf{z}^b$  are vectors of zeros if, respectively,  $a(y, \mathbf{x}, \boldsymbol{\theta}) = -\infty$  or  $b(y, \mathbf{x}, \boldsymbol{\theta}) = \infty$ . This claim follows since  $\mathbf{Z}$  is bounded and  $r$  is bounded. Indeed, since  $r$  is continuous, positive, integrates to one on  $\mathbb{R}$ , and is zero at the infinities, it is bounded on  $[-\infty, \infty]$ . We omit the arguments for second-order derivatives since they are very similar.  $\square$

**Lemma B.4.** *If, in Model (2) in the main text, the density  $r$  is strictly positive and continuously differentiable,  $\boldsymbol{\theta}_*$  is an interior point, and, for every  $\mathbf{t} \in \mathbb{R}^d$ , as  $n \rightarrow \infty$ ,*

$$\frac{1}{n} \sum_{i=1}^n \mathbb{E} \left[ \int_0^1 \{\nabla^2 \ell^i(\boldsymbol{\theta}_* + s\mathbf{t}/\sqrt{n}; Y_i, \mathbf{x}_i) - \nabla^2 \ell^i(\boldsymbol{\theta}_*; Y_i, \mathbf{x}_i)\} s ds \right] \rightarrow 0, \quad (1)$$

$$\frac{1}{n^2} \sum_{i=1}^n \text{var} \left\{ \int_0^1 \mathbf{t}^\top \nabla^2 \ell^i(\boldsymbol{\theta}_* + s\mathbf{t}/\sqrt{n}; Y_i, \mathbf{x}_i) \mathbf{t} s ds \right\} \rightarrow 0, \quad (2)$$

and

$$\frac{1}{n} \sum_{i=1}^n \text{cov}\{\nabla \ell^i(\boldsymbol{\theta}_*; Y_i, \mathbf{x}_i)\} = n^{-1} \mathcal{I}_n(\boldsymbol{\theta}_*; \mathbf{X}) \rightarrow \mathcal{I}(\boldsymbol{\theta}_*) \quad (3)$$

for some positive definite  $\mathcal{I}(\boldsymbol{\theta}_*)$ ; then

$$\sqrt{n}(\hat{\boldsymbol{\theta}}_n - \boldsymbol{\theta}_*) = \mathcal{I}(\boldsymbol{\theta}_*)^{-1} n^{-1/2} \sum_{i=1}^n \nabla \ell^i(\boldsymbol{\theta}_*; Y_i, \mathbf{x}_i) + o_{\mathbf{P}}(1).$$

*Proof.* We verify the conditions of Theorem 2.2 in Hjort and Pollard (2011) from which the conclusion follows. Define the remainder  $D_i$  in a linear approximation of  $\ell$  around the true parameter  $\boldsymbol{\theta}_*$  by

$$D_i = D_i(Y_i, \mathbf{x}_i, \mathbf{t}) = \ell^i(\boldsymbol{\theta}_* + \mathbf{t}; Y_i, \mathbf{x}_i) - \ell^i(\boldsymbol{\theta}_*; Y_i, \mathbf{x}_i) - \nabla \ell^i(\boldsymbol{\theta}_*; Y_i, \mathbf{x}_i)^\top \mathbf{t}.$$

The likelihood has continuous second order partial derivatives in some open ball around the interior  $\boldsymbol{\theta}_*$  because  $r$  is continuously differentiable, and hence we can use the mean value theorem with integral-form remainder to write, for all small enough  $\mathbf{t}$ ,

$$D_i = \mathbf{t}^\top \left[ \int_0^1 \nabla^2 \ell^i(\boldsymbol{\theta}_* + s\mathbf{t}; Y_i, \mathbf{x}_i) s \, ds \right] \mathbf{t}.$$

Now straightforward algebra shows (1) and (2) are equivalent to, respectively,  $\sum_{i=1}^n v_{i,0}(\mathbf{t}/\sqrt{n}) \rightarrow 0$ , where  $v_{i,0}(\mathbf{t}) = \mathbb{E}(D_i) - \mathbf{t}^\top \mathbb{E}\{\nabla^2 \ell^i(\boldsymbol{\theta}_*; Y_i, \mathbf{x}_i)\} \mathbf{t}$ , and  $\sum_{i=1}^n v_i(\mathbf{t}/\sqrt{n}) \rightarrow 0$ , where  $v_i(\mathbf{t}) = \text{var}(D_i)$ .  $\square$

*Remark.* By specializing the remarks following Theorem 2.2 in Hjort and Pollard (2011) to the present setting one sees that condition (3) can be weakened to

$$0 < \liminf_{n \rightarrow \infty} n^{-1} \lambda_{\min}\{\mathcal{I}_n(\boldsymbol{\theta}_*; \mathbf{X})\} \leq \limsup_{n \rightarrow \infty} n^{-1} \lambda_{\max}\{\mathcal{I}_n(\boldsymbol{\theta}_*; \mathbf{X})\} < \infty,$$

in which case the conclusion is

$$\mathcal{I}_n(\boldsymbol{\theta}_*; \mathbf{X})^{1/2}(\hat{\boldsymbol{\theta}} - \boldsymbol{\theta}_*) = \mathcal{I}_n(\boldsymbol{\theta}_*; \mathbf{X})^{-1/2} \nabla \ell_n(\boldsymbol{\theta}_*; \mathbf{Y}, \mathbf{X}) + o_{\mathbf{P}}(1).$$

**Lemma B.5.** *If  $r$  is continuously differentiable and Assumption 1 holds, then the family of Hessians*

$$\{\nabla^2 \ell^i(\cdot; y_i, \mathbf{x}_i) : i \in \mathbb{N}, y_i \in \mathcal{Y}_i, \mathbf{x}_i \in \mathcal{X}\}$$

*is equicontinuous at interior  $\boldsymbol{\theta}_*$ ; that is, for every  $\epsilon > 0$  there is a  $\delta = \delta_\epsilon > 0$  such that, for every  $i \in \mathbb{N}$ ,  $y_i \in \mathcal{Y}_i$ ,  $\mathbf{x}_i \in \mathcal{X}$ , and  $\boldsymbol{\theta}$  with  $\|\boldsymbol{\theta} - \boldsymbol{\theta}_*\| \leq \delta$ ,*

$$\|\nabla^2 \ell^i(\boldsymbol{\theta}; y_i, \mathbf{x}_i) - \nabla^2 \ell^i(\boldsymbol{\theta}_*; y_i, \mathbf{x}_i)\| \leq \epsilon.$$

*Proof.* Let  $\epsilon > 0$  be given and consider  $\boldsymbol{\theta} \in B_\delta(\boldsymbol{\theta}_*)$ , the open ball of radius  $\delta > 0$  centered at  $\boldsymbol{\theta}_*$ . Upon decreasing  $\delta$  if necessary we may assume all points in  $B_\delta(\boldsymbol{\theta}_*)$  are interior points of  $\Theta$ , so the Hessians exist on the ball.

Using that the spectral norm is sub-multiplicative, we get

$$\|\nabla^2 \ell^i(\boldsymbol{\theta}; y_i, \mathbf{x}_i) - \nabla^2 \ell^i(\boldsymbol{\theta}_*; y_i, \mathbf{x}_i)\| \leq \|\mathbf{Z}_i\| \|\mathbf{H}(y_i, \mathbf{x}_i, \boldsymbol{\theta}) - \mathbf{H}(y_i, \mathbf{x}_i, \boldsymbol{\theta}_*)\|.$$

Since  $d$  is fixed, Assumption 1 gives  $\|\mathbf{Z}_i\| \leq \sqrt{d} \|\mathbf{Z}_i\|_\infty \leq c_1$ . Consider  $y_i$  such that  $m_i^a(y_i, \mathbf{x}_i)$  and  $m_i^b(y_i, \mathbf{x}_i)$  are both finite and note  $\mathbf{H}(t_1, t_2)$  is, since  $r$  is continuously differentiable, uniformly continuous on the compact set given by Assumption 1. Thus, we have  $\|\mathbf{H}(y_i, \mathbf{x}_i, \boldsymbol{\theta}) - \mathbf{H}(y_i, \mathbf{x}_i, \boldsymbol{\theta}_*)\| \leq \epsilon/c_1$  uniformly in  $\mathbf{x}_i$  and  $\boldsymbol{\theta} \in B_\delta(\boldsymbol{\theta}_*)$  by picking  $\delta$  small enough. Similar arguments apply to  $y_i$  where one of the endpoints are infinite, so the conclusion is true for every  $y_i$ . Thus, since  $\mathcal{Y}$  is finite, it also holds uniformly in  $y_i$  and that completes the proof.  $\square$

*Proof of Theorem 2.* We start by verifying (1)–(2) in Lemma B.4. The former follows from Lemma B.5 which gives that for any  $\epsilon > 0$ , it holds for all large enough  $n$  that

$$\|\nabla^2 \ell^i(\boldsymbol{\theta}_* + st/\sqrt{n}; Y_i, \mathbf{x}_i) - \nabla^2 \ell^i(\boldsymbol{\theta}_*; Y_i, \mathbf{x}_i)\| \leq \epsilon$$

for all  $i \in \mathbb{N}$ ,  $Y_i \in \mathcal{Y}_i$ , and  $\mathbf{x}_i \in \mathcal{X}$ . Thus, the left-hand side in (1) is less than  $\epsilon$  for all large enough  $n$ , and hence so is its upper limit.

Now, using again the fact that the linear predictors, when they are finite, are contained in compact sets,  $\|\nabla^2 \ell^i(\boldsymbol{\theta}; Y_i, \mathbf{x}_i)\|$  is bounded uniformly in  $i \in \{1, 2, \dots\}$ ,  $Y_i \in \mathcal{Y}_i$ ,  $\mathbf{x}_i \in \mathcal{X}$ , and  $\boldsymbol{\theta} \in B_\delta(\boldsymbol{\theta}^*)$ , for small enough  $\delta > 0$ . Thus, there is a  $c_1 < \infty$  such that

$$\text{var} \left\{ \int_0^1 \mathbf{t}^\top \nabla^2 \ell^i(\boldsymbol{\theta}_* + s\mathbf{t}/\sqrt{n}; Y_i, \mathbf{x}_i) \mathbf{t} s \, ds \right\} \leq c_1$$

for all large enough  $n$ , and hence (2) holds. From this it also follows that the eigenvalues of  $n^{-1} \mathcal{I}_n(\boldsymbol{\theta}; \mathbf{X}) = -n^{-1} \sum_{i=1}^n \mathbb{E}\{\nabla^2 \ell^i(\boldsymbol{\theta}_*; Y_i, \mathbf{x}_i)\}$  are bounded. Thus, by remarks following Lemma B.4, we are done if we can establish a lower bound on the eigenvalues of  $n^{-1} \mathcal{I}_n(\boldsymbol{\theta}; \mathbf{X})$  and verify that

$$\mathcal{I}_n(\boldsymbol{\theta}_*; \mathbf{X})^{-1/2} \ell_n(\boldsymbol{\theta}_*; \mathbf{Y}, \mathbf{X}) \rightsquigarrow \mathcal{N}(0, \mathbf{I}_d).$$

This is straightforwardly done in two steps: first, for any  $\mathbf{t} \in \mathbb{R}^d$

$$\sum_{i=1}^n \mathbf{t}^\top \nabla \ell^i(\boldsymbol{\theta}_*; Y_i, \mathbf{x}_i) / \sqrt{\mathbf{t}^\top \mathcal{I}_n(\boldsymbol{\theta}_*; Y_i, \mathbf{x}_i) \mathbf{t}} \rightsquigarrow \mathcal{N}(0, 1)$$

by Lyapunov's central limit theorem, using that the elements of  $\nabla \ell^i(\boldsymbol{\theta}_*; Y_i, \mathbf{x}_i)$  are uniformly bounded and hence have uniformly bounded third (say) moment. Then, the conclusion follows from the Cramér-Wold theorem if  $0 < \liminf_{n \rightarrow \infty} n^{-1} \lambda_{\min}\{\mathcal{I}_n(\boldsymbol{\theta}_*; \mathbf{X})\} \leq \limsup_{n \rightarrow \infty} n^{-1} \lambda_{\max}\{\mathcal{I}_n(\boldsymbol{\theta}_*; \mathbf{X})\} < \infty$  (Biscio et al., 2018). We have already established the upper bound, so it only remains to show the lower bound holds. But Lemma B.2 implies  $\lambda_{\max}\{\nabla^2 \ell_n(\boldsymbol{\theta}_*; \mathbf{Y}, \mathbf{X})\} \leq -\epsilon \sum_{i=1}^n \mathbf{Z}_i^\top \mathbf{Z}_i$  for some  $\epsilon > 0$ . The lower bound follows by observing  $\mathcal{I}_n(\boldsymbol{\theta}_*; \mathbf{X}) = -\mathbb{E}\{\nabla^2 \ell_n(\boldsymbol{\theta}_*; \mathbf{Y}, \mathbf{X})\}$ , and that completes proof.  $\square$

*Proof of Corollary 1.* Let us first prove that Assumption 1 is satisfied, starting with the first

part. Recall that in the model in Example 2, when  $\sigma = 1$  is known,

$$\mathbf{Z}_i = -[\mathbf{x}_i, \mathbf{x}_i]^\top; \quad \mathbf{m}_i = [t_j^i, t_{j+1}^i]^\top,$$

with the first or second row of  $\mathbf{Z}_i$  replaced by zeros if, respectively,  $t_j^i = -\infty$  or  $t_{j+1}^i = \infty$ . Because  $\mathcal{Y}$  is finite, there is an  $\epsilon > 0$  such that  $t_j^i \leq t_{j+1}^i + \epsilon$  for all  $i$  and  $j$ . Thus, for any fixed  $y_i$  with finite endpoints, the image of the map  $(\mathbf{x}_i, \boldsymbol{\beta}) \mapsto \mathbf{Z}_i \boldsymbol{\beta} + \mathbf{m}_i$  is contained in the set  $T = \{\mathbf{t} \in \mathbb{R}^2 : t_1 \leq t_2 + \epsilon\}$ . Moreover, that map is continuous and hence maps the compact set  $\{\mathbf{x}_i : \|\mathbf{x}_i\|_\infty \leq c_1\} \times \{\boldsymbol{\beta} \in \mathbb{R}^p : \|\boldsymbol{\beta} - \boldsymbol{\beta}_*\|_1 \leq \rho\}$  to a compact set, say  $E_i \subseteq T$ . Because  $\mathcal{Y}$  is finite, there finitely many  $E_i$ , so their union is a compact subset of  $T$ , which shows the first part of Assumption 1 holds. The second part is immediate from  $\|\mathbf{x}_i\|_\infty \leq c_1$  and  $\mathcal{Y}$  being finite.

The proof is completed by observing, since  $\mathbf{Z}_i = -[\mathbf{x}_i, \mathbf{x}_i]^\top$ , we have  $\mathbb{E}(\mathbf{Z}_i^\top \mathbf{Z}_i) = \mathbf{Z}_i^\top \mathbf{Z}_i = 2\mathbf{x}_i \mathbf{x}_i^\top$ , and  $\liminf_{n \rightarrow \infty} \lambda_{\min} \{\sum_{i=1}^n \mathbb{E}(\mathbf{Z}_i^\top \mathbf{Z}_i)/n\} > 0$  if and only if  $\liminf_{n \rightarrow \infty} \lambda_{\min} \{\mathbf{X}^\top \mathbf{X}/n\} > 0$ .

□

**Theorem B.6.** *Under the conditions of Theorem 2 in the main text, if in addition  $r$  is twice continuously differentiable, then as  $n \rightarrow \infty$ ,*

$$\left\| -n^{-1} \nabla^2 \ell_n(\widehat{\boldsymbol{\theta}}_n; \mathbf{Y}, \mathbf{X}) - n^{-1} \mathcal{I}_n(\boldsymbol{\theta}; \mathbf{X}) \right\| \rightarrow 0$$

*in probability, and hence*

$$\left\{ -\nabla^2 \ell_n(\widehat{\boldsymbol{\theta}}_n; \mathbf{Y}, \mathbf{X}) \right\}^{1/2} (\widehat{\boldsymbol{\theta}}_n - \boldsymbol{\theta}_*) \rightsquigarrow \mathcal{N}(\mathbf{0}, \mathbf{I}_d).$$

*Proof.* The convergence in distribution follows from Theorem 2.2 and Slutsky's theorem once the convergence in probability is established. To do this, it suffices because  $\widehat{\boldsymbol{\theta}}_n$  is consistent

to show, in probability,

$$\sup_{\boldsymbol{\theta} \in B} \left\| -n^{-1} \nabla^2 \ell_n(\boldsymbol{\theta}; \mathbf{Y}, \mathbf{X}) - n^{-1} \mathcal{I}_n(\boldsymbol{\theta}_*) \right\| \rightarrow 0$$

where  $B = \{\boldsymbol{\theta} \in \mathbb{R}^d : \|\boldsymbol{\theta} - \boldsymbol{\theta}_*\|_1 \leq \rho\}$  and  $\rho$  is chosen small enough that  $B \subseteq \Theta$  and to satisfy Assumption 1. To get this we verify the conditions of Theorem 8.2 by Pollard (1990). Pick an arbitrary element of  $\nabla^2 \ell^i(\boldsymbol{\theta}; Y_i, \mathbf{x}_i)$  and, to simplify notation, denote it  $f_i(Y_i, \boldsymbol{\theta})$ . By arguments in the proof of Theorem 2,  $f_i(Y_i, \boldsymbol{\theta})$  is bounded by some  $c_1 < \infty$ , uniformly in  $i \in \mathbb{N}$ ,  $Y_i \in \mathcal{Y}_i$  and  $\boldsymbol{\theta} \in B$ . Thus, in Pollard's notation, we have the envelope  $F_i = c_1$ , so his condition (i) holds. Also, if  $\mathbf{F}_n$  is the vector with elements  $F_i$ ,  $\|\mathbf{F}_n\|_1 = nc_1$ . Now, since  $r$  is twice continuously differentiable, derivatives of  $f_i$  with respect to  $\boldsymbol{\theta}$  are continuous. Thus, by arguments essentially the same as those in the proof of Theorem 2, upon increasing  $c_1$  if necessary, we have  $\|\nabla_{\boldsymbol{\theta}} f_i(Y_i, \boldsymbol{\theta})\|_\infty \leq c_1$ . We will use this to, as required by Pollard's condition (ii), bound the  $L_1$ -packing number for balls of radius  $\epsilon \|\mathbf{F}_n\|_1 = \epsilon nc_1$  of the set

$$\mathcal{F}_n(Y) = \{\mathbf{f}_n(\mathbf{Y}, \boldsymbol{\theta}) = [f_1(Y_1, \boldsymbol{\theta}), \dots, f_1(Y_1, \boldsymbol{\theta})]^\top : \boldsymbol{\theta} \in B\} \subseteq \mathbb{R}^n.$$

If  $\boldsymbol{\theta}_1$  and  $\boldsymbol{\theta}_2$  are two points in  $B$ , then for some  $\tilde{\boldsymbol{\theta}}$  between them,

$$\begin{aligned} \|\mathbf{f}_n(\mathbf{Y}, \boldsymbol{\theta}_1) - \mathbf{f}_n(\mathbf{Y}, \boldsymbol{\theta}_2)\|_1 &= \sum_{i=1}^n |f_i(Y_i, \boldsymbol{\theta}_1) - f_i(Y_i, \boldsymbol{\theta}_2)| \\ &= \sum_{i=1}^n |\nabla_{\boldsymbol{\theta}} f_i(Y_i, \tilde{\boldsymbol{\theta}})^\top (\boldsymbol{\theta}_1 - \boldsymbol{\theta}_2)| \\ &\leq nc_1 \|\boldsymbol{\theta}_1 - \boldsymbol{\theta}_2\|_1, \end{aligned}$$

where the second line is by Taylor's theorem with Lagrange-form remainder, and the last line uses that the gradient is bounded by  $c_1$  on  $B$ . Thus, an  $\epsilon$ -cover of  $B$  translates to an  $nc_1\epsilon$ -cover of  $\mathcal{F}_n(Y)$ . But the  $\epsilon$ -covering number of  $B$  is less than  $(\rho + 2\rho/\epsilon)^d$  (Wainwright, 2019, Example 5.8), and hence the  $nc_1\epsilon$ -packing number of  $\mathcal{F}_n(Y)$  is less than  $(\rho + 4\rho/\epsilon)^d$

(Wainwright, 2019, Lemma 5.5). Since  $\log\{(\rho + 4\rho/\epsilon)^d\} = o(n)$  we have verified Pollard's condition (ii), and that completes the proof.  $\square$

### B.3 Asymptotics with diverging number of parameters

We will use the framework of Negahban et al. (2012) to prove Theorem 4.1. To that end we establish a concentration inequality for the gradient of the objective function and a restricted strong convexity.

**Lemma B.7.** *If  $r$  is continuous and strictly positive on  $\mathbb{R}$  and Assumption 1 holds, then there exists a  $c_1$  such that, for any  $t \geq 0$ ,*

$$\mathbb{P}(\|\nabla G_n(\boldsymbol{\theta}_*; \mathbf{Y}, \mathbf{X})\|_\infty > t) \leq 2d \exp(-c_1 n t^2)$$

*Proof.* The gradient at  $\boldsymbol{\theta}_*$  exists and is continuous since  $r$  is continuous. Thus, using that the linear predictors are contained in compact sets when they are finite (Assumption 1), the summands in  $\nabla G_n(\boldsymbol{\theta}_*; \mathbf{Y}, \mathbf{X}) = -n^{-1} \sum_{i=1}^n \nabla \ell^i(\boldsymbol{\theta}_*, Y_i, \mathbf{x}_i)$  are uniformly bounded by some  $c_2 < \infty$  by the arguments in the proof of Theorem 2 (there applied to the Hessian). We then get by Hoeffding's inequality, using that the gradient has mean zero by Lemma B.3, for  $j \in \{1, \dots, d\}$ ,

$$\mathbb{P}(|[\nabla G_n(\boldsymbol{\theta}_*; \mathbf{Y}, \mathbf{X})]_j| > t) \leq 2 \exp\left(-\frac{2nt^2}{c_2^2}\right).$$

Thus, by a union bound (sub-additivity of measures),

$$\mathbb{P}(\|\nabla G_n(\boldsymbol{\theta}_*; \mathbf{Y}, \mathbf{X})\|_\infty > t) \leq 2d \exp\left(-\frac{2nt^2}{c_2^2}\right),$$

which finishes the proof.  $\square$

**Lemma B.8.** *Let  $\bar{B}_M$  denote the closed ball of radius  $M$  centered at the origin in  $\mathbb{R}^d$ . If  $\boldsymbol{\theta}_*$  is  $s$ -sparse and  $\|\boldsymbol{\theta}_*\|_\infty \leq c_1$ , then for small enough  $M > 0$ , there exists a  $\kappa_M > 0$  not depending on  $n$  or  $p$  such that, for  $\boldsymbol{\Delta} \in \mathbb{C}(S) \cap \bar{B}_M$  and realizations  $(\mathbf{Y}, \mathbf{X})$  in the event*

$\mathcal{C}_{\kappa,n,p}$  in Theorem 4.1,

$$G_n(\boldsymbol{\theta}_* + \boldsymbol{\Delta}; \mathbf{Y}, \mathbf{X}) - G_n(\boldsymbol{\theta}_*; \mathbf{Y}, \mathbf{X}) - \nabla G_n(\boldsymbol{\theta}_*; \mathbf{Y}, \mathbf{X})^\top \boldsymbol{\Delta} \geq \kappa_M \|\boldsymbol{\Delta}\|^2.$$

*Proof.* Continuity of the derivative of  $r$  ensures  $\nabla^2 G_n(\cdot; \mathbf{Y}, \mathbf{X})$  is continuous, and hence, by the mean-value theorem, the left-hand side in the inequality to be established is equal to

$$\boldsymbol{\Delta}^\top \nabla^2 G_n(\boldsymbol{\theta}_* + \tilde{\boldsymbol{\Delta}}; \mathbf{Y}, \mathbf{X}) \boldsymbol{\Delta} / 2$$

for some  $\tilde{\boldsymbol{\Delta}}$  on the line connecting 0 and  $\boldsymbol{\Delta}$ . Let  $\tilde{\boldsymbol{\theta}} = \boldsymbol{\theta}_* + \tilde{\boldsymbol{\Delta}}$ . It now suffices to show that  $\mathbf{H}_{11}(y_i, \mathbf{x}_i, \tilde{\boldsymbol{\theta}})$ ,  $\mathbf{H}_{22}(y_i, \mathbf{x}_i, \tilde{\boldsymbol{\theta}})$ , and  $\lambda_{\min}\{\mathbf{H}(y_i, \mathbf{x}_i, \tilde{\boldsymbol{\theta}})\}$  are bounded away from zero when, respectively,  $b_i(y_i, \mathbf{x}_i, \tilde{\boldsymbol{\theta}}) = \infty$ ,  $a_i(y_i, \mathbf{x}_i, \tilde{\boldsymbol{\theta}}) = -\infty$ , and both are finite. But this follows from Lemma B.2 since  $\|\tilde{\boldsymbol{\theta}} - \boldsymbol{\theta}_*\|_1 = \|\tilde{\boldsymbol{\Delta}}\|_1 \leq \|\boldsymbol{\Delta}\|_1 \leq 4\|\boldsymbol{\Delta}_S\|_1 \leq sM$ , and we can pick  $M$  small enough that Assumption 1 holds with  $\rho = sM$ .  $\square$

Before giving a proof of Theorem 3 we recall Corollary 1 of Negahban et al. (2012) and specialize it to our setting in the following lemma.

**Lemma B.9.** *If  $\lambda_n > 2\|\nabla G_n(\boldsymbol{\theta}_*)\|_\infty$  and conditions (a)–(d) of Theorem 3 hold, then there exists  $c_1, c_2 < \infty$  such that for large enough  $n$ ,  $d$ , and every outcome in the set  $\mathcal{C}_{\kappa,n,d}$ ,  $\|\hat{\boldsymbol{\theta}}_n^\lambda - \boldsymbol{\theta}_*\| \leq c_1 \lambda_n^2$  and  $\|\hat{\boldsymbol{\theta}}_n^\lambda - \boldsymbol{\theta}_*\|_1 \leq c_2 \lambda_n$ .*

*Proof.* Condition (G1) in (Negahban et al., 2012) is satisfied because  $\|\cdot\|_1$  is a norm. Theorem 1 and Lemma B.8 show their condition (G2) is satisfied on any compact ball centered at the origin, which is sufficient (Negahban et al., 2012, p. 9). More specifically, pick an  $M \in (0, \infty)$  and note that for any  $\boldsymbol{\Delta} \in \mathbb{C}(S) \cap B_M$  it holds that (Negahban et al., 2012, Supplementary Material, p.29)

$$G_n^\lambda(\boldsymbol{\theta}_* + \boldsymbol{\Delta}) \geq G_n^\lambda(\boldsymbol{\theta}_*) + \kappa_M \|\boldsymbol{\Delta}\|^2 - 3\sqrt{s}\lambda_n \|\boldsymbol{\Delta}\|/2.$$

Thus for all large enough  $n$  and  $d$  and  $\boldsymbol{\Delta} \in \mathbb{C}(S) \cap \{\|\boldsymbol{\Delta}\| = M\}$ , since  $\lambda_n = o(1)$ ,  $G_n^\lambda(\boldsymbol{\theta}_* + \boldsymbol{\Delta}) > G_n^\lambda(\boldsymbol{\theta}_*)$ . Hence, by convexity,  $\|\hat{\boldsymbol{\theta}}_n^\lambda - \boldsymbol{\theta}_*\| \leq M$ . Because  $\|\boldsymbol{\theta}_*\|$  is bounded as  $d$  varies, this

shows  $\hat{\boldsymbol{\theta}}_n^\lambda$  is in a compact ball of fixed radius for all large enough  $n$  and  $d$ . The proof of Theorem 1 in Negahban et al. (2012) now applies almost verbatim, with the “global”  $\kappa_{\mathcal{L}}$  (their notation) replaced by the  $\kappa_M$  given by Lemma B.8.  $\square$

*Proof of Theorem 3.* By Lemma B.7 we can pick  $\lambda_n^2 = c_2 \log(d)/n$  and have that the probability of the event  $\mathcal{A}_{n,d} = \{(\mathbf{Y}, \mathbf{X}) : \|\nabla G_n(\boldsymbol{\theta}_*; \mathbf{Y}, \mathbf{X})\|_\infty > 2\lambda_n\}$  is upper bounded by  $2 \exp\{-c_6 n \lambda_n + \log(d)\}$  for all  $n$  and  $d$  and some  $c_6 > 0$ . Thus, by picking large enough  $c_2$  we get that  $\mathcal{A}_{n,d}$  happens with probability at most  $d^{-c_3}$  for some  $c_3 > 0$ . Thus, the result follows from Lemma B.9 and noting that  $P(\mathcal{C}_{\kappa,n,d} \cap \mathcal{A}_{n,d}^c) = P(\mathcal{C}_{\kappa,n,d}) - P(\mathcal{C}_{\kappa,n,d} \cap \mathcal{A}_{n,d}) \geq P(\mathcal{C}_{\kappa,n,d}) - d^{-c_3}$ , and that completes the proof.  $\square$

## B.4 Convergence of algorithm

*Proof of Theorem 4.* We check the conditions of Theorem 2 by Byrd et al. (2016). The termination criteria ensure the descent property  $G_n^\lambda(\boldsymbol{\theta}^k) \geq G_n^\lambda(\boldsymbol{\theta}^{k+1})$  (Byrd et al., 2016, p.5). Moreover, under either of conditions (a) and (b)  $G_n^\lambda$  is strictly convex by Theorem 2.1. Thus, for any starting value  $\boldsymbol{\theta}^0$ , the sequence of iterates are contained in a large enough compact ball  $B$  centered at  $\hat{\boldsymbol{\theta}}$ , which under condition (b) exists because  $G_n^\lambda$  is strongly convex. We have by continuity and strict convexity that  $\sup_{\boldsymbol{\theta} \in B} \|\nabla G_n(\boldsymbol{\theta}) + \lambda_2 \boldsymbol{\theta}\| < \infty$ ,  $\inf_{\boldsymbol{\theta} \in B} \lambda_{\min}\{\nabla^2 G_n(\boldsymbol{\theta}) + \lambda_2 \mathbf{I}_d\} > 0$ , and  $\sup_{\boldsymbol{\theta} \in B} \lambda_{\max}\{\nabla^2 G_n(\boldsymbol{\theta}) + \lambda_2 \mathbf{I}_d\} < \infty$ . The bound on the gradient implies the required Lipschitz-continuity and the eigenvalue bounds imply the eigenvalues of  $\nabla^2 G_n(\boldsymbol{\theta}^k) + \lambda_2 \mathbf{I}_d$  are bounded away from zero and from above for all  $k \in \{1, 2, \dots\}$ , which completes the proof.  $\square$

## References

Archer, K. J. and Williams, A. A. A. (2012). L1 penalized continuation ratio models for ordinal response prediction using high-dimensional datasets. *Statistics in Medicine* **31**, 1464–1474.

- Biscio, C. A. N., Poinas, A., and Waagepetersen, R. (2018). A note on gaps in proofs of central limit theorems. *Statistics & Probability Letters* **135**, 7–10.
- Boyd, S. P. and Vandenberghe, L. (2004). *Convex Optimization*. Cambridge University Press, Cambridge, UK ; New York.
- Byrd, R. H., Nocedal, J., and Oztoprak, F. (2016). An inexact successive quadratic approximation method for L-1 regularized optimization. *Mathematical Programming* **157**, 375–396.
- Folland, G. B. (2007). *Real Analysis: Modern Techniques and Their Applications*. Wiley, New York, second edition.
- Hjort, N. L. and Pollard, D. (2011). Asymptotics for minimisers of convex processes.
- Kroenke, K. and Spitzer, R. L. (2002). The PHQ-9: A new depression diagnostic and severity measure. *Psychiatric Annals* **32**, 509–515.
- Negahban, S. N., Ravikumar, P., Wainwright, M. J., and Yu, B. (2012). A unified framework for high-dimensional analysis of M-estimators with decomposable regularizers. *Statistical Science* **27**,.
- Pollard, D. (1990). Empirical processes: Theory and applications. *NSF-CBMS Regional Conference Series in Probability and Statistics* **2**, i–86.
- Prékopa, A. (1973). On logarithmic concave measures and functions. *Acta Scientiarum Mathematicarum* **34**, 335–343.
- Wainwright, M. J. (2019). *High-Dimensional Statistics: A Non-Asymptotic Viewpoint*. Cambridge University Press, Cambridge, UK.
